# Supplementary material for: Deep Learning, Machine Learning, Advancing Big Data Analytics and Management
Source: arXiv:2412.02187 source file (2024-12-03)
Supplement: Supplementary file 1 [file appendix.tex]

\part{Appendix}
